# Supplementary material for: Strain-induced enhancement of the charge-density-wave in the kagome metal ScV$_6$Sn$_6$
Source: arXiv:2403.18046 ancillary file (2024-03-26)
Supplement: Supplementary file 1 [file Strain_and_CDW_in_ScV6Sn6.pdf]

# Supplemental material for: Strain-induced enhancement of the charge-density-wave in the kagome metal $ScV_6Sn_6$


Manuel Tuniz**,[1] Armando Consiglio**,[2,3] Ganesh Pokharel,[4] Fulvio Parmigiani,[1,5] Titus Neupert,[6] Ronny Thomale,[2] Giorgio Sangiovanni,[2] Stephen D. Wilson,[4] Ivana Vobornik,[3] Federico Salvador,[3] Federico Cilento,[5] Domenico Di Sante,[7,8] and Federico Mazzola[3,9]

[1]*Dipartimento di Fisica, Universita degli studi di Trieste, 34127, Trieste, Italy*

[2]*Institut für Theoretische Physik und Astrophysik and Würzburg-Dresden Cluster of Excellence ct.qmat, Universität Würzburg, 97074 Würzburg, Germany*

[3]*Istituto Officina dei Materiali, Consiglio Nazionale delle Ricerche, Trieste I-34149, Italy*

[4]*Materials Department, University of California Santa Barbara, Santa Barbara, California 93106, USA*

[5]*Elettra - Sincrotrone Trieste S.C.p.A., Strada Statale 14, km 163.5, Trieste, Italy*

[6]*Physik-Institut, Universität Zürich, Winterthurerstrasse 190, CH-8057 Zürich, Switzerland*

[7]*Department of Physics and Astronomy, University of Bologna, 40127 Bologna, Italy*

[8]*Center for Computational Quantum Physics, Flatiron Institute, 162 5th Avenue, New York, NY 10010, USA*

[9]*Department of Molecular Sciences and Nanosystems, Ca' Foscari University of Venice, 30172 Venice, Italy*



(Dated: March 25, 2024)

** These authors contributed equally

## I. DETERMINATION OF THE AMPLITUDE MODE FREQUENCY FOR DIFFERENT DEGREES OF STRAIN

In order to study the evolution of the amplitude mode frequency we analyzed the Fourier Transform of the coherent part of the $\Delta R/R$ signal which has been isolated by fitting and removing the incoherent part of the signal. To do so we modeled the temporal of the incoherent part of the $\Delta R/R$ signal after the arrival of the pump pulse (time zero, t = 0) as [1, 2]:

$$\frac{\Delta R}{R}(t, t_{pp}) = G(t) \otimes \left[ A_1^e \, e^{-t/\tau_1^e} + A_2^e \, e^{-t/\tau_2^e} + B \right], \tag{1}$$

where $t_{pp}$ is the delay between the two pump pulses while G(t) represents the cross correlation between the pump and probe pulses, which turns to be ≈ 150 fs. $A_i^e$ denotes the amplitude of the electronic relaxation phenomena with time constant $\tau_i^e$. B represents the amplitude of much slower process (likely related to the heating of the sample) that in our time window can be approximated by a constant term.

In Fig. S1 is shown the Fourier Transform of the coherent part of the $\Delta R/R$ as a function of temperature for three different degrees of compressive strain.

It is worth nothing that the coherent part of the $\Delta R/R$ signal, being directly linked to the CDW amplitude mode, is expected to be the most direct probe of the effect of a lattice strain on the CDW order of the system. Conversely, the incoherent part of the signal, being primarily determined by the relaxation of hot electrons throughout the first Brillouin zone, constitutes a less effective probe of the effect of the lattice strain on the CDW order, and has not been considered in this analysis.

## II. STRAIN QUANTIFICATION FROM THE DEVICE GEOMETRY

The device we used to deliver strain is a molybdenum block with clamps. One clamp is fixed, one is activated by a screw. Thus, By rotating the screw of a fixed amount, we

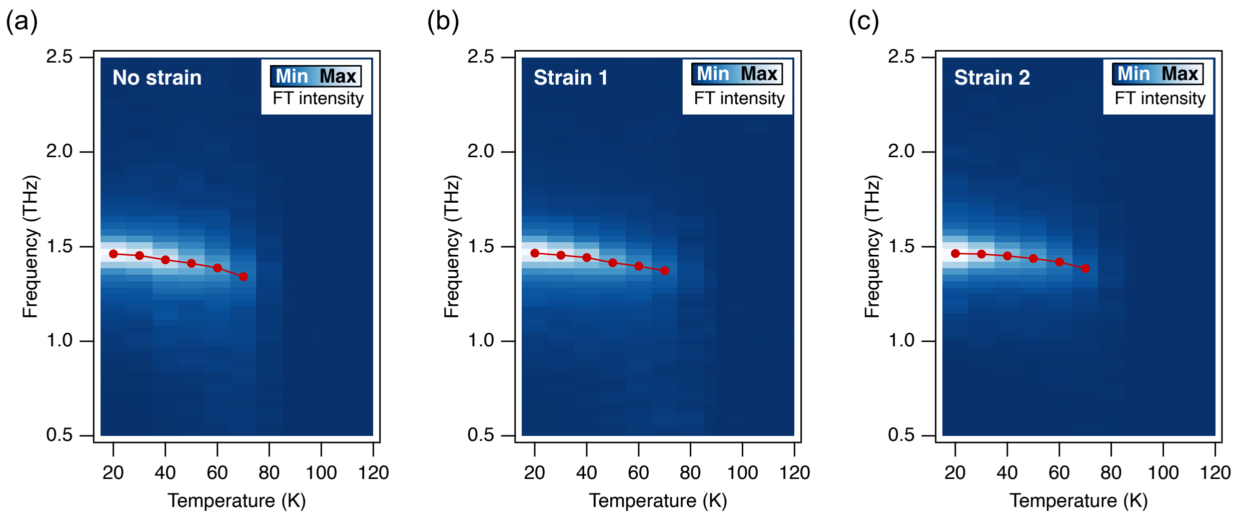


FIG. S1. Fourier transform of the coherent part of the $\Delta R/R$ signal for three different degrees of compressive strain: (a) no strain, (b) strain 1, (c) strain 2. The red traces show the center position of the peak and are compared in Fig. 2 of the main manuscript.

are able to deliver a certain strain to the plate on which the sample is glued, as described in the main text. One important problem in estimating the strain is that the compression delivered to the plate is not transferred exactly with the same strength to the sample, thus making difficult a quantification of this effect. This is the reason for which we preferred comparing the experiment to the theory. However, we report here a very crude methodology able to give us an upper limit of the strain delivered, including the fact that the plate has a finite thickness, which we call $2\tau$ in Fig.S2a. The methodology consist in calculating the deformation $\epsilon$ defined as the ratio of half of the plate thickness ($\tau$) and the bending radius $R$. This quantity can be estimated by various photographs and after by reporting on vector-graphics the resulting device and geometry as in Fig.S2b (reported for the strongest strain). This methodology has been already used various times to estimate the strain, as for example in the recent work by Liu et al. [3]. In our case, which is the best we can do with this methodology, the estimated strain corresponds to 2.4%. We stress again that this quantification is crude and is reported for completeness to show the strain gradient imposed by our geometry.

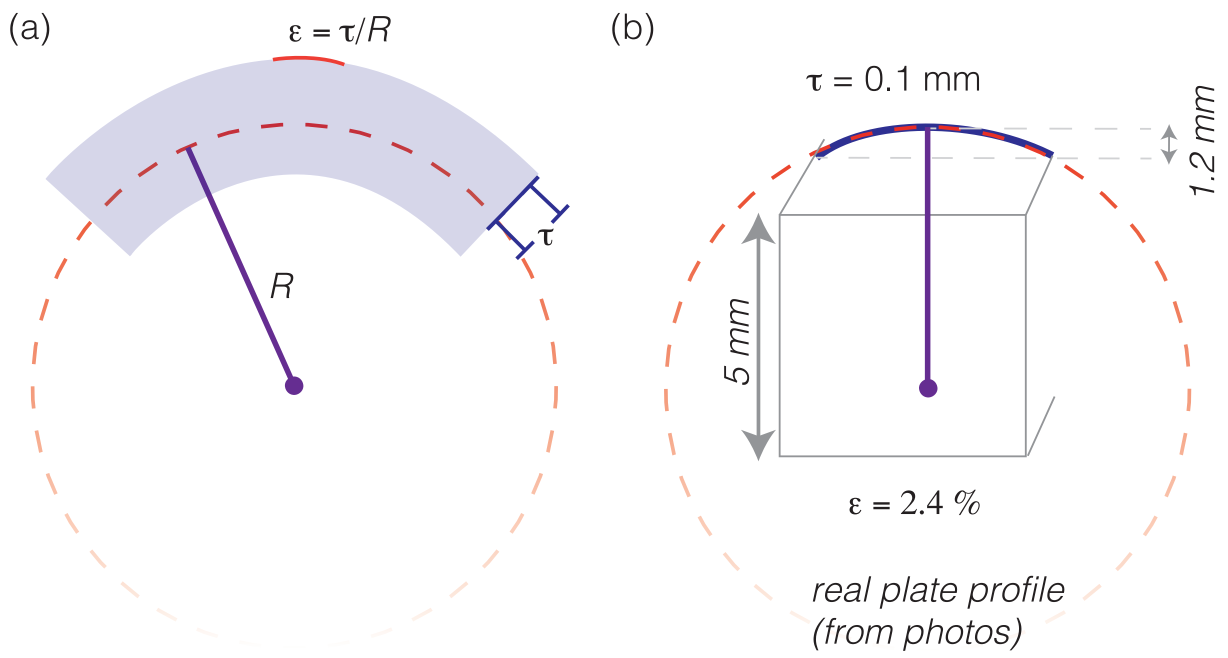


FIG. S2. (a) Strain methodology determined by the plate thickness and the bending radius. (b) Vector graphic of the real (maximum strain) situation extracted by various photographs. Here, the upper limit is quantified to be approximately 2.4%, likely the strain transferred to the sample is reduced.

## III. UNI-AXIAL STRAIN TUNING OF CDW-PHASE ELECTRONIC STRUCTURE

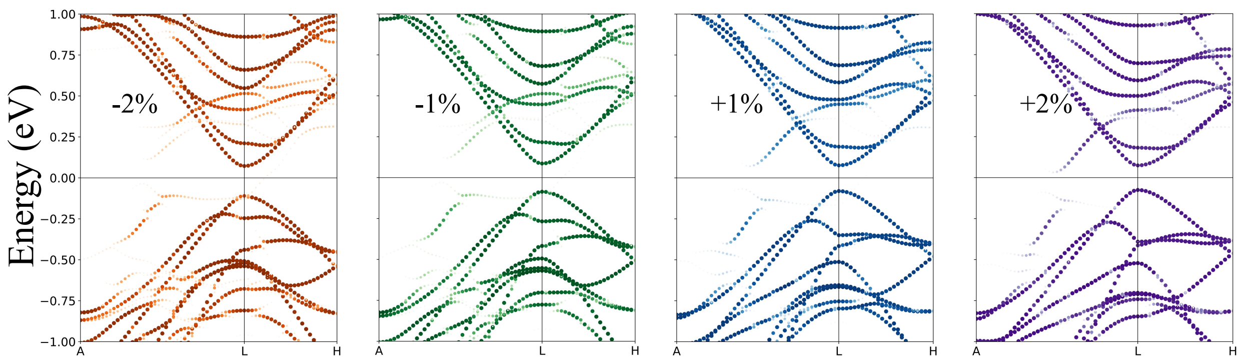


FIG. S3. Electronic band structure of the CDW geometry as a function of different percentages of uni-axial strain. The gap computed in panel 3(d) of the main text are obtained midway between the A and L high-symmetry points.

[1] Tuniz, M. *et al.* Ultrafast all-optical manipulation of the charge-density wave in $VTe_2$. *Phys. Rev. Res.* **5**, 043276 (2023). URL https://link.aps.org/doi/10.1103/PhysRevResearch.5.043276.

[2] Soranzio, D., Peressi, M., Cava, R. J., Parmigiani, F. & Cilento, F. Ultrafast broadband optical spectroscopy for quantifying subpicometric coherent atomic displacements in $WTe_2$. *Phys. Rev. Res.* **1**, 032033 (2019). URL https://link.aps.org/doi/10.1103/PhysRevResearch.1.032033.

[3] Liu, J. *et al.* Controllable strain-driven topological phase transition and dominant surface-state transport in $HfTe_5$. *Nature Communications* **15**, 332 (2024). URL https://doi.org/10.1038/s41467-023-44547-7.
